# Supplementary material for: Precise Experimental Test of the Luttinger Theorem and Particle-Hole Symmetry for a Strongly Correlated Fermionic System
Source: arXiv:2007.10208 ancillary file (2020-07-20)
Supplement: Supplementary file 1 [file Supplemental_Material.pdf]

# Supplemental Material: Precise Experimental Test of the Luttinger Theorem and Particle-Hole Symmetry for a Strongly Correlated Fermionic System

Md. Shafayat Hossain, M. A. Mueed, M. K. Ma, K. A. Villegas Rosales, Y. J. Chung, L. N. Pfeiffer, K. W. West, K. W. Baldwin, and M. Shayegan
*Department of Electrical Engineering, Princeton University, Princeton, New Jersey 08544, USA*
(Dated: July 14, 2020)

## I. EXPERIMENTAL DETAILS

Our samples are two-dimensional electron systems (2DESs) confined to modulation-doped, GaAs/AlGaAs heterostructures, grown by molecular beam epitaxy. We studied samples from two different wafers. The 2DESs in these samples have densities ($n$) ranging from 10.16 to 2.20 (in units of $10^{10}$ cm$^{-2}$), and are buried 190 nm underneath the surface to ensure high quality. The low-temperature mobilities of our samples are in the range $1.1 - 0.5$ (in units of $10^7$ cm$^2$/Vs) which are very high and therefore favorable to ballistic transport of composite fermions (CFs). This is a crucial requirement for observing the CF geometric resonance (GR) features.

For our measurements, Hall bar samples were fabricated using standard photolithography techniques, and alloyed InSn contacts were used to contact the 2DESs. The samples comprise multiple Hall bar sections, each of length 100 $\mu$m and width 50 $\mu$m. Via electron-beam lithography and using a negative electron-beam resist (TEBN-1), we patterned the sample surface with one-dimensional, strain-inducing superlattices perpendicular to the current direction [1–3]. Thanks to the piezoelectric effect in GaAs, the periodic strain from this surface superlattice propagates to the 2DES and leads to a weak density modulation. The availability of multiple sections enables us to study different superlattice periods in the same sample. The different sections are patterned with periods ranging from 190 to 225 nm. Lastly, we fit each sample with an In back gate to tune the electron density *in-situ*.

We note that the period of the superlattice required to observe clear GR features depends on the electron density and the depth of the 2DES. This is because CFs are extremely fragile and require a gentle modulation to exhibit clear GR features. In our samples, the depth of the 2DES is fixed and equals 190 nm. On the other hand, we control the density via applying voltage bias to the back gate. Therefore, in order to observe clear GR features at all the densities in our experiments, we use superlattices of different periods depending on the electron density. For densities down to $n \simeq 7.05$, we observe clear GR features for $a = 225$ and 200 nm. For lower densities we use $a = 200$ nm (for $n \simeq 6.99$ to 5.34) and $a = 190$ nm (for $n = 5.57$ to 2.26) to ensure an appropriate modulation.

The experiments were carried out using a lock-in technique, and in a $^3$He cryostat with a base temperature of 0.3 K. We passed a current ($I = 10$ nA, 13 Hz) perpendicular to the density modulation for transport measurements.

## II. FERMI SEA IN INTERACTING VS. NON-INTERACTING SYSTEMS

The Luttinger theorem states that the area of the Fermi sea remains unaffected by the interaction so long as there is no phase transition. However, is it the electron or the hole density that determines the Fermi sea? For non-interacting carriers in semiconductors, there can be two plausible answers: The area of the Fermi sea can be determined by the majority carriers, or the minority carriers. In doped semiconductors, it is known that it is the minority carriers that determine the area of the Fermi sea: In $n$-doped systems, the area of the Fermi sea is determined by the density of electrons in the conduction band while in $p$-doped systems, where the valence band is almost full, the Fermi sea area is determined by the density of the empty states in the valence band, i.e., "holes," rather than electrons. In strongly correlated systems, the physics of the Fermi sea can be more intricate. For instance, in three-dimensional high-$T_c$ cuprate superconductors, the volume of the Fermi surface for large hole dopings ($x$) relative to the half-filled band (where there is a Mott insulator phase), is determined by the number of holes $(1 + x)$ [4, 5], i.e., the majority carriers. Strangely, however, at low hole dopings, the volume of the Fermi surface appears to be $x$ rather than the number of holes $(1+x)$ or electrons $(1-x)$ [6]. Such subtlety in the Fermi surface is yet to be understood.

The Fermi sea of CFs that we study in our measurements offers a simple and useful insight to the Luttinger physics. CFs form in the lowest Landau level (LL), a prototypical flatband system where no kinetic energy is present and the Coulomb energy dominates the physics. Nevertheless, when the lowest LL is half-filled, a Fermi sea of CFs emerges out of interaction instead of the Mott insulator phase observed in cuprates. (In the half-filled LL, there is a magnetic field present that explicitly breaks the time-reversal symmetry; this is in contrast to the Mott insulator where the half-filled flatband preserves the time-reversal symmetry in the absence of a magnetic field.) We examine the CF Fermi sea via geometric

resonance measurements by directly probing the Fermi wave vector $k_F^*$. Following our discussion in the main text, as we measure $k_F^*$ away from the half-filled LL, we find that among the two choices for the Fermi sea: small (from minority carriers) or large (from majority carriers), CFs choose the small one. Particle-hole symmetry about $\nu = 1/2$ (that we find to hold for CFs) further dictates that the Fermi seas for $\nu < 1/2$ and $\nu > 1/2$ are both small. This is similar to the non-interacting semiconductor systems, and apparently different from the cuprates.

Here we also elaborate on the description of Fig. 3 (of the main text) plots in the context of the Luttinger theorem. As briefly described in the main text, since the CFs are formed from electron and flux quanta, all the interactions should be contained in the CF quasiparticles themselves, and CFs should behave as non-interacting particles [7]. However, it turns out that this is not true, and there is always some residual interaction between the CFs [7]. One can tune the strength of this interaction by controlling the CF density. As we lower the density of our 2DES, the Coulomb energy ($E_{\mathrm{Coul}} = e^2/4\pi\varepsilon l_B$) at a fixed filling decreases as $B^{-1/2}$. On the other hand, the cyclotron energy ($E_{\mathrm{Cyc}} = \hbar eB/m^*$) at the same filling goes as $B$. This means that the ratio of these two energies, $\kappa = E_{\mathrm{Coul}}/E_{\mathrm{Cyc}}$ at the same filling increases as $B^{-1/2}$, i.e. as $n^{-1/2}$, as we lower the density $n$. This parameter $\kappa$ (shown in the top axes of Figs. 3-4, S2, and S4 plots), the so-called LL mixing parameter, is a measure of the inter-CF interaction strength. Mixing with the higher LLs that have nodes in their wavefunctions results in a substantial enhancement of the residual interaction between the CFs. Such mixing and the resulting interaction between the CFs affect the CF ground state significantly at low fillings. They can lead, e.g., to a transition to a CF Wigner crystal [8]. Thus, just by tuning the 2DES density over a large range and measuring the CF Fermi wave vector, we can investigate the effect of inter-CF interaction on the CF Fermi sea area. Figure 3 of the main text shows such $k_F^*$ data and it is clear from the plots that $k_F^*$, which determines the CF Fermi sea area, follows the same expression $k_F^* = (4\pi n_{\mathrm{min}})^{1/2}$ over a large range of electron density and LL mixing, making a convincing case that the Luttinger theorem is obeyed in a strongly interacting system.

## III. POSITIONS OF GEOMETRIC RESONANCE MINIMA AND PARTICLE-HOLE SYMMETRY ABOUT $\nu = 1/2$

### III.1. General discussion

According to the CF theory [7, 9, 10], the flux-electron CFs ignore the large, external magnetic field ($B$) and only experience an *effective* magnetic field $B^* = B - B_{\nu=1/2}$, where $B_{\nu=1/2}$ is the field at $\nu = 1/2$, $\nu = hn/eB$ is the LL filling factor, and $n$ is the 2DES density. Near $\nu = 1/2$ CFs execute cyclotron motion in a small $B^*$, similar to their electron counterparts near $B = 0$ [1, 7, 10–14]. This phenomenon enables us to directly probe the CF Fermi sea via measurements of CF Fermi wave vector. We use a GR technique in 2DESs with an imposed, small, periodic density modulation [Fig. 2(a)]. The working principle of GR is straightforward and requires no fitting parameters. The CFs' cyclotron orbit in a small $B^*$ has radius $R_c^* = \hbar k_F^*/eB^*$, the size of which is determined by the magnitude of the CFs' Fermi wave vector, $k_F^*$ [1, 7, 10–14]. If the CFs have a long mean-free-path so they can complete a cyclotron orbit without scattering, then a GR occurs when the orbit diameter becomes commensurate with the period ($a$) of the density modulation [Fig. 2(a)]. Quantitatively, it is generally assumed that, when $2R_c^*/a = i + 1/4$ ($i = 1, 2, 3, ...$), GRs manifest as minima in magneto-resistance at $B_i^*$ according to the following equation [1, 13, 14]:

$$\frac{2\hbar k_F^*}{e|B_i^*|}\frac{1}{a} = (i + \frac{1}{4}). \tag{S1}$$

In the main text, we considered three plausible cases while determining the expected positions of the CF GR minima:

(i) The density of CFs is fixed as a function of $B$ and is equal to the density of the electrons, i.e., $k_F^* = (4\pi n)^{1/2}$.

(ii) The density of CFs is equal to the density of the minority carriers in the lowest LL, namely $k_F^* = (4\pi n_{\mathrm{min}})^{1/2}$, where $n_{\mathrm{min}} = n$ for $\nu < 1/2$, and $n_{\mathrm{min}} = n(1-\nu)/\nu$ (i.e., the density of holes in the lowest LL) for $\nu > 1/2$.

(iii) The density of CFs is equal to half the number of flux quanta penetrating the sample, i.e., $n^* = B/(2h/e)$, if the CFs are Dirac fermions. This means $k_F^* = l_B^{-1}$ [where $l_B = (\hbar/eB)^{1/2}$ is the magnetic length]. The Dirac CF theory thus predicts that $k_F^*$ should change with $B$ according to $k_F^* = (4\pi n)^{1/2} \times (B_{i=1}/B_{\nu=1/2})^{1/2}$. The Halperin-Lee-Read [10] theory also predicts a magnetic length dependence in $k_F^*$ according to $k_F^* = l_B^{-1} = (4\pi n)^{1/2} \times (B_{i=1}/B_{\nu=1/2})^{1/2}$.

In the following subsections, we elaborate on how we obtain the $\nu$ and $B_{i=1}^*$ positions of the CF GR features as well as the $k_F^*$ of CFs for cases (i) to (iii).

### III.2. Fixed-density model

This is the simplest assumption and assumes that the density of CFs is equal to the density of the electrons, i.e., $n^* = n$. This means $k_F^*$ simply equals $(4\pi n)^{1/2}$. The fixed-density model predicts the expected positions for the CF GR to be $B_i^* = 2\hbar(4\pi n)^{1/2}/ea(i + 1/4)$ [see Eq. (S1)]. Therefore, the magnetic field positions for the CF

GR minima are:

$$B^{\pm(i)}_{\text{fixed}} = B_{\nu=1/2} \pm \frac{2\hbar(4\pi n)^{1/2}}{ea(i+1/4)}. \tag{S2}$$

This directly results in the expected filling factor positions of the GR minima:

$$\nu^{\pm(i)}_{\text{fixed}} = \left[2 \mp \frac{2}{a(i+\frac{1}{4})(\pi n)^{1/2}}\right]^{-1}. \tag{S3}$$

We use the above two equations along with $k^*_F = (4\pi n)^{1/2}$ to obtain the blue markings in Figs. 2(c, d), S1, and the blue curves in Figs. 3, S2, and S4.

### III.3. Minority-carrier model

According to the minority-carrier model, the density of CFs is equal to the density of the minority carriers in the lowest LL, implying that $k^*_F = (4\pi n_{\text{min}})^{1/2}$, where $n_{\text{min}} = n$ for $\nu < 1/2$, and $n_{\text{min}} = n(1-\nu)/\nu$ (i.e., the density of holes in the lowest LL) for $\nu > 1/2$. The expression $k^*_F = (4\pi n_{\text{min}})^{1/2}$ can be rewritten as:

$$k^*_F = \begin{cases} (2\nu)^{1/2} l_B^{-1}; & \nu < 1/2 \\ [2(1-\nu)]^{1/2} l_B^{-1}; & \nu > 1/2 \end{cases} \tag{S4}$$

It is clear from Eq. (S4) that, the $k^*_F$ of CFs on the two sides of $\nu = 1/2$ will be equal if $l_B$ is fixed. We use Eq. (S4) to obtain the red curves in Figs. 3, S2 (a, b), and S4.

Now, we work out an expression for the filling factor positions of the GR minima. For a given GR minimum for $\nu < 1/2$, we have $B^* = B - B_{\nu=1/2} = B - 2\nu B = B(1-2\nu)$ where $B$ is the magnetic field position of the GR minimum. Then, using Eq. (S1), we find:

$$\frac{2\hbar k^*_F}{eB(1-2\nu)}\frac{1}{a} = \frac{2k^*_F l_B^2}{1-2\nu}\frac{1}{a} = (i+\frac{1}{4}). \tag{S5}$$

Using $k^*_F l_B = (2\nu)^{1/2}$ that we show in Eq. (S4) for $\nu < 1/2$, we obtain a quadratic equation for the $\nu$ where the GR minimum occurs for the minority-carrier model ($\nu_{\text{min}}$):

$$\frac{(2\nu_{\text{min}})^{1/2}}{1-2\nu_{\text{min}}} = \frac{a}{2l_B}(i+\frac{1}{4}). \tag{S6}$$

On the other hand, in the case of a GR minimum for $\nu > 1/2$, $|B^*| = -B^* = B(2\nu-1)$ and $k^*_F l_B = [2(1-\nu)]^{1/2}$ [Eq. (S4)]. Therefore, the GR minima occur when:

$$\frac{[2(1-\nu_{\text{min}})]^{1/2}}{2\nu_{\text{min}}-1} = \frac{a}{2l_B}(i+\frac{1}{4}). \tag{S7}$$

Note that, the left-hand sides of Eqs. (S6) and (S7) are related by the particle-hole transformation $\nu \leftrightarrow (1-\nu)$ about $\nu = 1/2$ and thereby:

$$\frac{(2\nu_{\text{min}})^{1/2}}{1-2\nu_{\text{min}}} \leftrightarrow \frac{[2(1-\nu_{\text{min}})]^{1/2}}{2\nu_{\text{min}}-1}. \tag{S8}$$

This means that, if $\nu$ is a solution of Eq. (S6), then $(1-\nu)$ is a solution of Eq. (S7), provided that $a/l_B$ is fixed. Therefore, particle-hole symmetry emerges within the minority-carrier model and the mirror symmetry in GR can be visualized when $\nu_{\text{GR}}$ on the two sides of $\nu = 1/2$ are compared at a fixed $a/l_B$. Indeed, solving Eqs. (S6) and (S7), we find:

$$\nu^{\pm(i)}_{\text{min}} = \frac{1}{2} \pm \frac{\left[\left(i+\frac{1}{4}\right)^2\left(\frac{a}{l_B}\right)^2 + 1\right]^{1/2} - 1}{\left(i+\frac{1}{4}\right)^2\left(\frac{a}{l_B}\right)^2}, \tag{S9}$$

which is symmetric with respect to $\nu = 1/2$ at a fixed $a/l_B$. We use Eq. (S9) to obtain the red markings in Figs. 2(d), S1(b), and the red curves in Figs. 4 and S2(c).

Using Eq. (S9), we can derive an expression for the magnetic field positions of the GR minima:

$$B^{\pm(i)}_{\text{min}} = B_{\nu=1/2}\left[1 \mp 2\frac{\left[\left(i+\frac{1}{4}\right)^2\left(\frac{a}{l_B}\right)^2 + 1\right]^{1/2} - 1}{\left(i+\frac{1}{4}\right)^2\left(\frac{a}{l_B}\right)^2}\right]^{-1}. \tag{S10}$$

We use Eq. (S10) to obtain the red markings in Figs. 2(c), S1(a), and the red curves in Fig. S2(d).

### III.4. Dirac theory

According to the Dirac theory, the density of CFs is half the number of flux quanta penetrating the sample, i.e., $n^* = B/(2h/e)$. This means $k^*_F = l_B^{-1}$ [where $l_B = (\hbar/eB)^{1/2}$ is the magnetic length]. The Dirac CF theory thus predicts that $k^*_F$ should change with $B$ according to $k^*_F = (4\pi n)^{1/2} \times (B_{i=1}/B_{\nu=1/2})^{1/2}$. We use this expression to obtain the green curves in Figs. 3, S2 (a, b), and S4.

Here, we work out the expressions for GR minima in terms of $\nu$ and $B$ expected from the Dirac theory, using the calculations by Cheung *et al.* [15]. Following the Dirac CF theory, Cheung *et al.* [15] determined the locations of the GR minima as a function of the electron density $n$ as follows (see Eq. (3.7) of Ref. [15]):

$$n^{\pm(i)}_{\text{Dirac}} = \frac{B}{2\phi_0} \pm \frac{(\hbar B/e)^{1/2}}{(i+\frac{1}{4})a\phi_0}, \tag{S11}$$

where $n^{\pm}_{\text{Dirac}}$ are the GR positions around $\nu = 1/2$ as one sweeps $n$ at a fixed magnetic field $B$, and $B_{\nu=1/2} = 2\phi_0 n$ where $\phi_0 = h/e$. We can rewrite Eq. (S11) in terms of $\nu$ as:

$$\nu^{\pm(i)}_{\text{Dirac}} = \frac{1}{2} \pm \frac{1}{\left(i+\frac{1}{4}\right)\left(\frac{a}{l_B}\right)}. \tag{S12}$$

We use Eq. (S12) to obtain the green markings in Figs. 2(d), S1(b), and the green curves in Figs. 4 and S2(c).

Cheung *et al.* [15] also worked out the magnetic field positions of the CF GR features based on the Dirac theory. The result is as follows (see Eq. (3.5) of Ref. [15]):

$$B^{\pm(i)}_{\rm Dirac}(i) = B_{\nu=1/2}\left[1+2\frac{1\pm\left(1+(i+\frac{1}{4})^2a^2(4\pi n)\right)^{1/2}}{(i+\frac{1}{4})^2a^2(4\pi n)}\right], \tag{S13}$$

We use Eq. (S13) to obtain the green markings in Figs. 2(c), S1(a), and the green curves in Fig. S2(d).

### III.5. Halperin-Lee-Read theory

The Halperin-Lee-Read theory [10] also predicts a magnetic length dependence in $k_F^*$ according to $k_F^* = l_B^{-1} = (4\pi n)^{1/2} \times (B_{i=1}/B_{\nu=1/2})^{1/2}$. Cheung *et al.* [15] carefully calculated the positions of the GR minima according to the Halperin-Lee-Read description of the CF Fermi sea, incorporating the corrections from the unscreened electric field produced by the surface superlattice that we use in our GR measurements. This residual electric field renders small corrections with an opposite sign for $\nu$ larger or smaller than 1/2. Cheung *et al.* find (see Eq. (3.20) of Ref. [15]):

$$n^{\pm(i)}_{\rm HLR} = n^{\pm(i)}_{\rm Dirac} \pm \frac{B}{2\phi_0}\frac{\left(\frac{2}{(1+4i)\pi^{1/2}}\right)^3}{a^3\left(\frac{B}{2\phi_0}\right)^{3/2}}. \tag{S14}$$

Rewriting this expression in terms of $\nu$ yields:

$$\nu^{\pm(i)}_{\rm HLR} = \nu^{\pm(i)}_{\rm Dirac} \pm \frac{1}{2\left(i+\frac{1}{4}\right)^3\left(\frac{a}{l_B}\right)^3}, \tag{S15}$$

and

$$B^{\pm(i)}_{\rm HLR} = B^{\pm(i)}_{\rm Dirac} \pm B_{\nu=1/2}\left[\frac{1}{a(i+\frac{1}{4})(4\pi n)^{1/2}}\right]^3. \tag{S16}$$

We use Eqs. (S15) and (S16) to obtain the brown markings in Fig. S1 and the brown curves in Figs. S2(c, d). It is clear that the $\nu$ positions of the GRs from Eqs. (S12) and (S15) are symmetric about $\nu = 1/2$, similar to Eq. (S9). This corroborates the fact that both the Dirac and Halperin-Lee-Read theories predict particle-hole symmetry about $\nu = 1/2$ at a fixed $a/l_B$. Moreover, $\nu^{\pm}_{\rm Dirac}$ and $\nu^{\pm}_{\rm HLR}$ (i.e., $B^{\pm}_{\rm Dirac}$ and $B^{\pm}_{\rm HLR}$) are essentially the same for our experimental $a/l_B$ values to within 1%.

## IV. COMPARISON WITH THE EXPERIMENTAL DATA

In this Section, we compare our experimental data vis-à-vis predictions from different theories.

We start by showing in Fig. S1 the CF GR features for six densities plotted as a function of $B$ [Fig. S1(a)] and $\nu$ [Fig. S1(b)], similar to the plots in Figs. 2(c, d) of the main text. In the main text, we compare our data with the fixed-density and minority-carrier models, as well as the Dirac theory. Here in Fig. S1, we also add markings indicating the *expected* positions of the $i = 1$ CF GR minima, according to the predictions of the Halperin-Lee-Read theory. In Fig. S1(a), except for the fixed-density model, all the models and theories predict GR positions that are asymmetric about $B^* = 0$. The predicted positions in Fig. S1(b) are also asymmetric with respect to $\nu = 1/2$. Clearly, in all traces, the positions of the observed GR minima agree best with the red marks, i.e., with the assumption that $k_F^*$ is determined by the minority-carrier density. It is also clear from Fig. S1 plots that the differences between the observed GR minima positions and the predictions from all the models and theories are easily discernible from the experimental traces.

Figure S2 captures a comprehensive summary of the experimental data, including the predictions from all the models and theories discussed in Section III. In Figs. S2 (c, d), we plot $\nu_{\rm GR}$ and $B^*_{i=1}$ taken directly from the experimental traces, and we use the simple expression $k_F^* = (5/4)eaB^*_{i=1}/2\hbar$ to obtain experimental $k_F^*$ values for Figs. S2(a, b) plots. In order to test our data against cases (i)-(iii), we plot the predictions form the fixed-density model (blue curves), minority-carrier model (red curves), Dirac (green curves), and Halperin-Lee-Read (brown curves) theories. One important finding in Fig. 4 [and Fig. S2(c)] plots is that the experimental GR data, when plotted in terms of $\nu_{\rm GR}$ vs. $a/l_B$, are symmetric with respect to $\nu = 1/2$ in the entire density range. Importantly, in the $k_F^*$ vs. $a/l_B$ plot of Fig. S2(b), there is also a mirror symmetry. However, as seen in Fig. S2(d), there are subtle asymmetries in $B^*_{i=1}$ about $B^* = 0$ even if the data are plotted as a function of $a/l_B$. We also note that, for clarity, we are not including in Fig. S2 the $a = 225$ nm data shown in Figs. (2-4) of the main text.

The plots in Fig. S2 and their comparison with different models and theories allow us to draw the following important conclusions:

(A) The ***minority-carrier model*** [case (ii), red curves], that we find to obey the Luttinger theorem and particle-hole symmetry, agrees best with the experimental data in all the Fig. S2 plots.

(B) The ***fixed-density model*** [case (i), blue curves] does not correctly reproduce the experimental data. Although for the $\nu < 1/2$ side, the predictions of this model are exactly the same as the case (ii), for $\nu > 1/2$, the predictions deviate most from the observed positions of the GR minima.

(C) In contrast, the Dirac (green curves) and Halperin-Lee-Read theories (brown curves) show deviations from the experimental data. The reason for this difference is straightforward. The expression $k_F^* = (2\nu)^{1/2}l_B^{-1}$ for

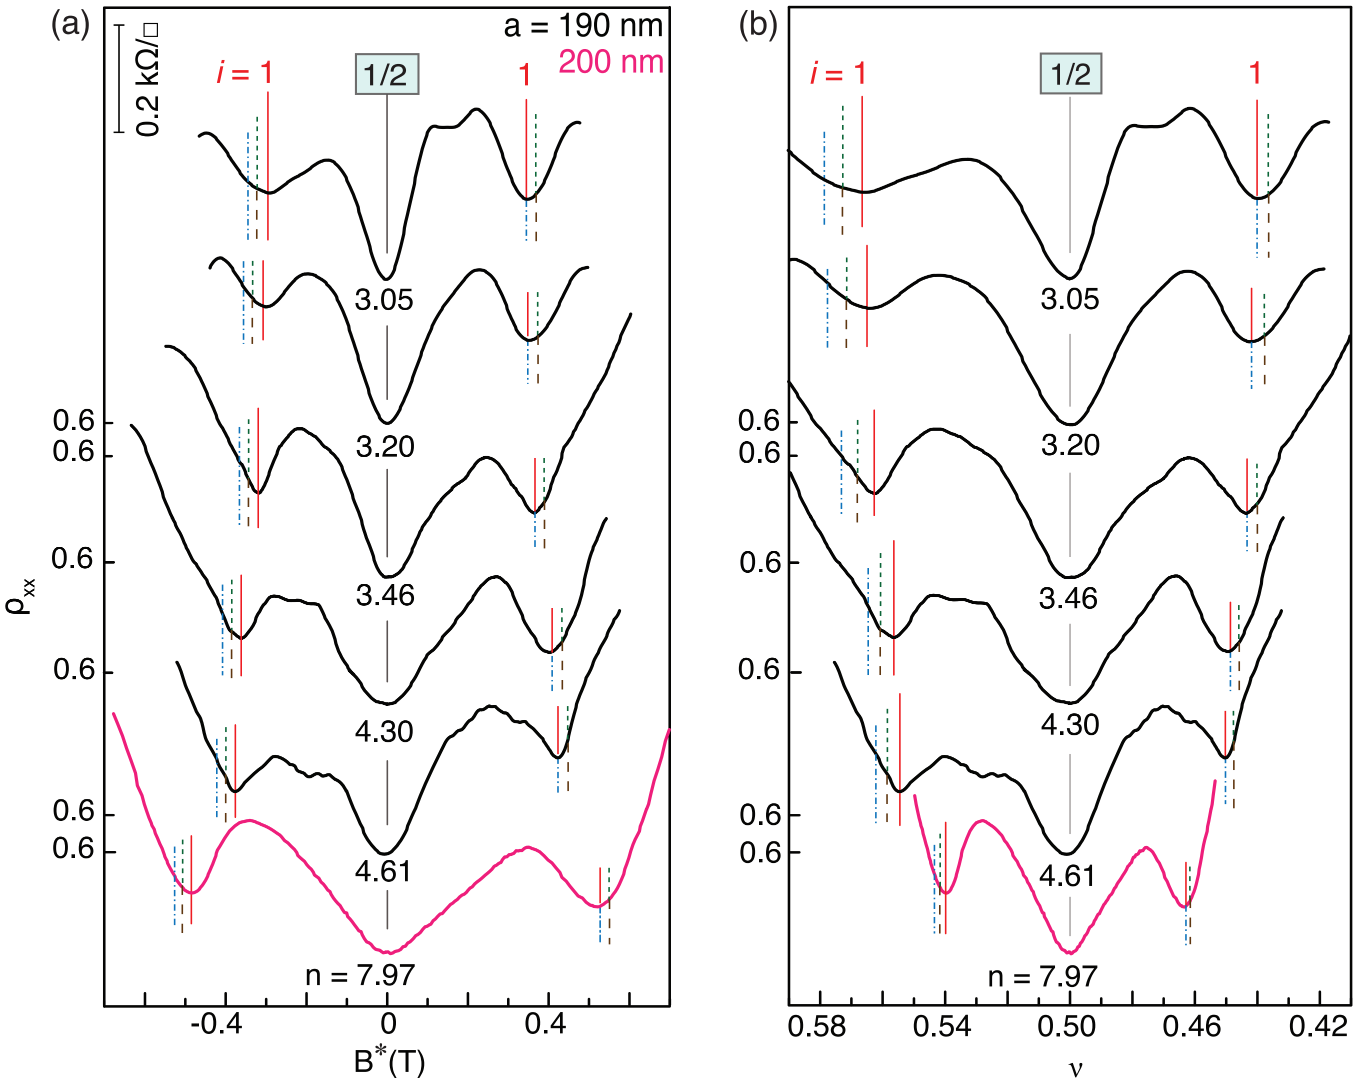


FIG. S1. (a) and (b): Plots similar to Figs. 2(c, d) of the main text, demonstrating the CF GR features plotted as a function of $B^*$ and $\nu$, respectively, and their comparison with the predictions of different assumptions. Traces are shown for six densities, as marked for each trace. The traces are for $a = 190$ nm (black) and 200 nm (magenta). Vertical (dash-dotted) blue, (solid) red, (short-dashed) green, and (long-dashed) brown lines mark the *expected* positions for the $i = 1$ GR for fully spin-polarized CFs according to the fixed density model, minority-carrier model, Dirac, and Halperin-Lee-Read theories, respectively. The blue and red lines coincide for $\nu < 1/2$ ($B^* > 0$). Also, the blue lines in (a) are exactly symmetric in their positions with respect to $B^* = 0$. The experimental data best match the predictions of the minority-carrier model (red vertical lines). The differences between the observed minima positions and the predictions from the fixed density model, Dirac, and Halperin-Lee-Read theories are well discernible.

$\nu < 1/2$ [shown in Eq. (S4)] means that $k_F^*$ is constant ($= (4\pi n)^{1/2}$) when $\nu < 1/2$ and is independent of magnetic field. The Dirac CF theory, on the other hand, predicts $k_F^* = l_B^{-1}$, implying that, away from $\nu = 1/2$, $k_F^*$ is not fixed for a fixed $n$ and changes with field, namely, $k_F^* = (4\pi n)^{1/2} \times (B/B_{\nu=1/2})^{1/2}$. In addition, when $\nu > 1/2$, Dirac CF theory predicts the same $k_F^* = l_B^{-1}$ whereas the minority-carrier model and the experimental data point towards $k_F^* = [2(1-\nu)]^{1/2}/l_B$. A recently proposed theory [16], however, suggests that the discrepancy with the experimental data can be resolved within the ***Dirac/Halperin-Lee-Read*** framework if one incorporates subtle effects, such as electrostatic contribution of the applied modulation, gauge-field fluctuations, etc. It adds a bit of complexity to the theory to explain the data, whereas a much simpler ***minority-carrier model*** appears to bring out the underlying physics.

(D) The correction factor to obtain the predictions of Halperin-Lee-Read theory from the Dirac is extremely small. Therefore, the predictions of the two theories (Dirac and Halperin-Lee-Read) are essentially the same (see Fig. S2).

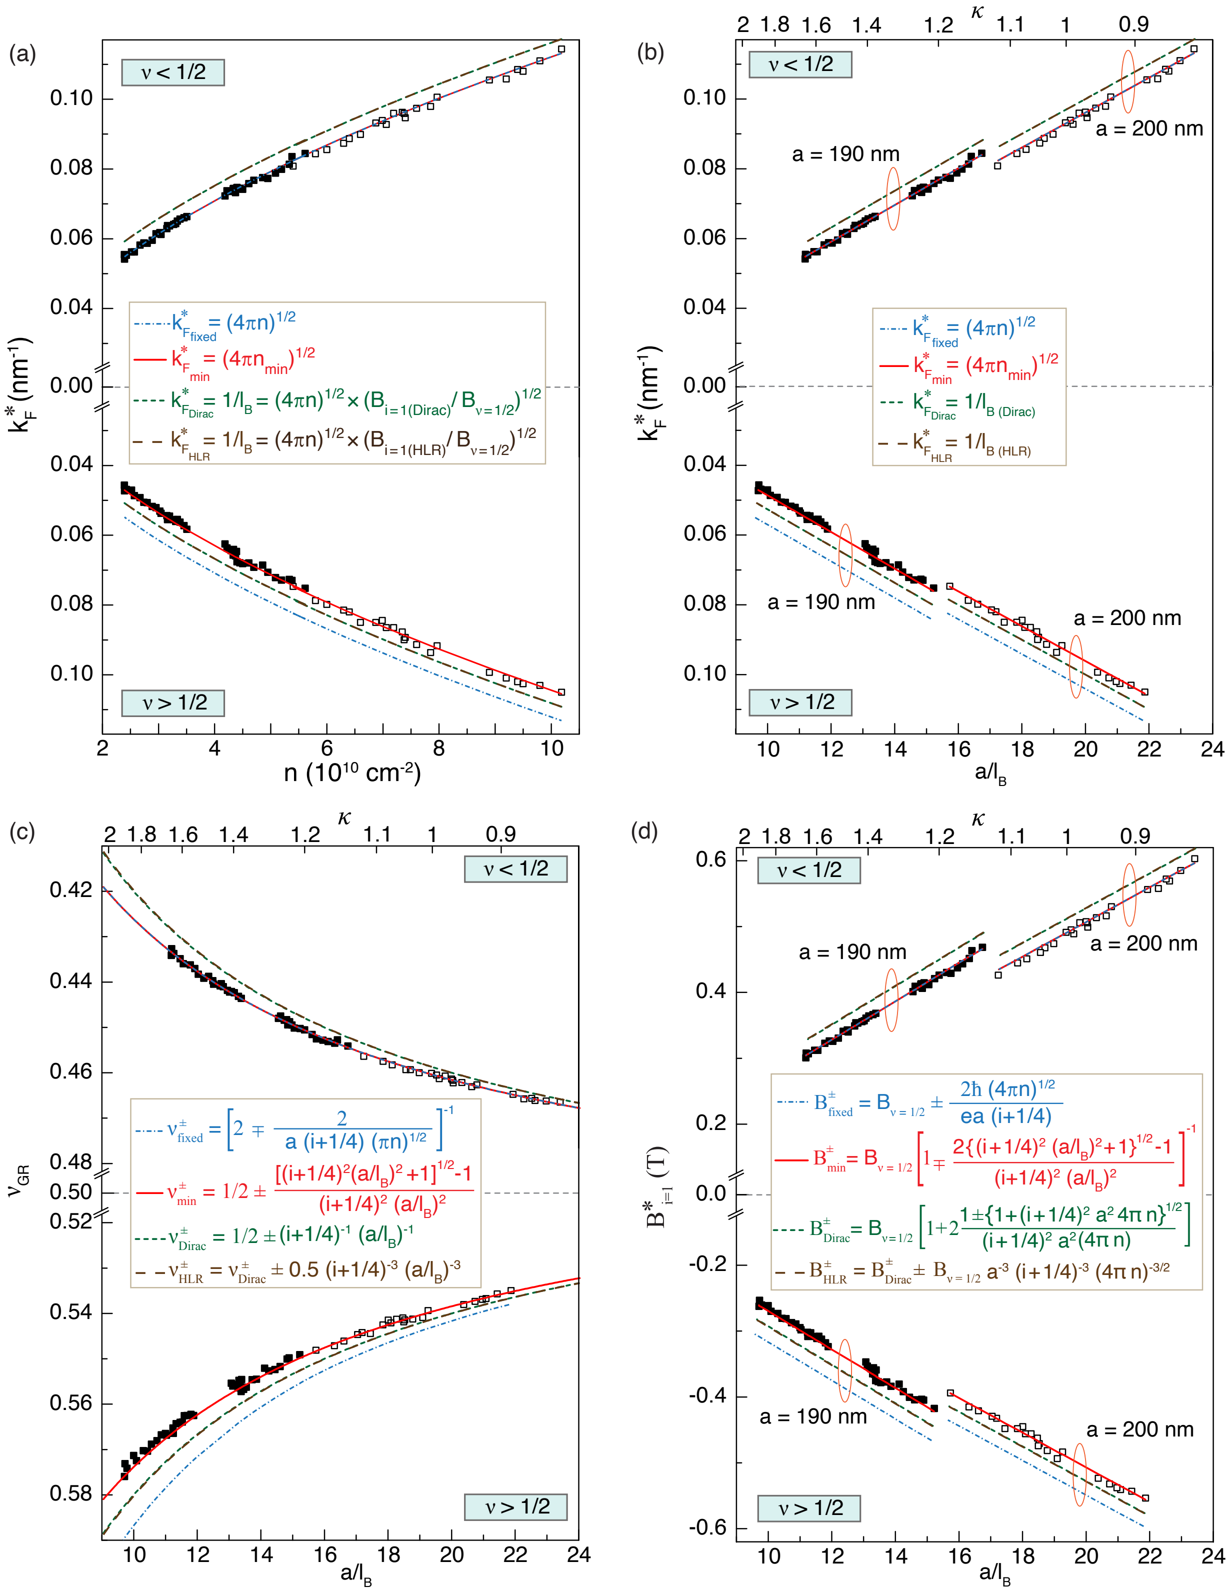


FIG. S2. (a) The CF Fermi wave vector plotted against density $n$, asserting that $k_F^* = (4\pi n^*_{\min})^{1/2}$ (red curves) is a reasonable representation of the data. (b) The CF Fermi wave vector, (c) filling-factor and (d) effective field positions of the observed CF GR minima at different densities, plotted against $a/l_B$ and LL mixing parameter $\kappa$ (top axes). The closed and open symbols represent experimental data from two different samples with $a = 190$ nm and $a = 200$ nm, respectively. The Blue, red, green, and brown curves are the predictions of the fixed-density model, minority-carrier model, Dirac, and Halperin-Lee-Read theories, respectively. For each model/theory, the results of calculations are shown in different ranges of $a$ where the experimental data were taken.

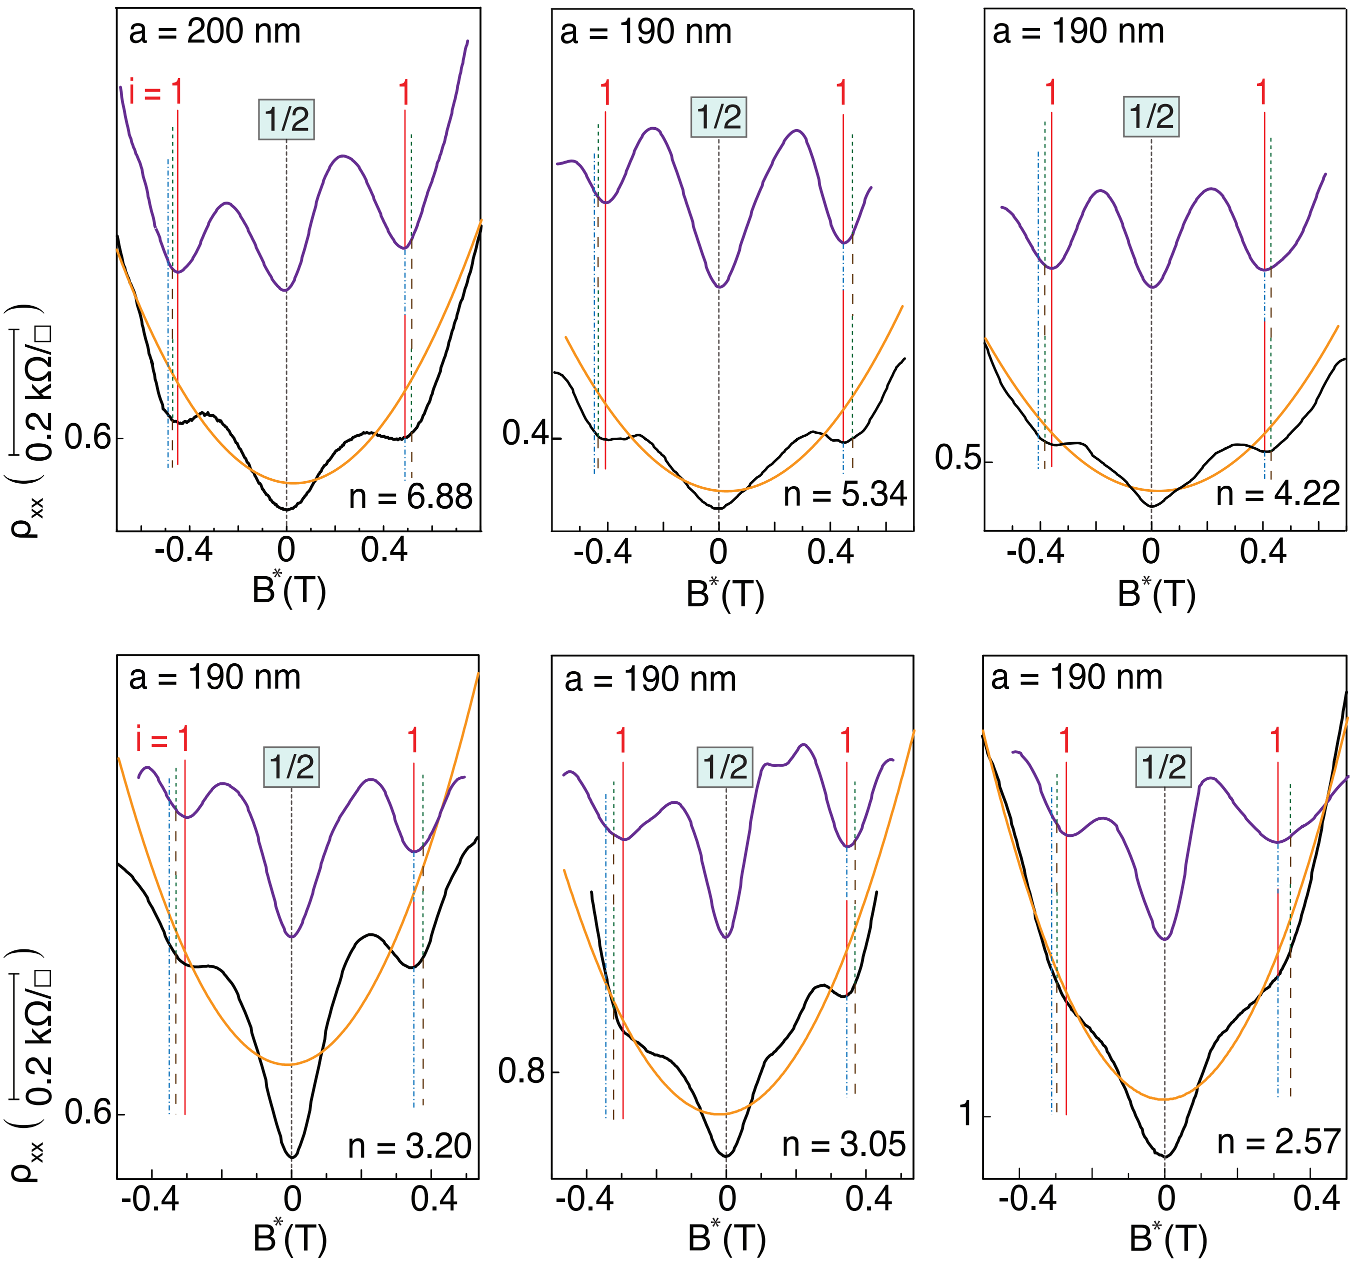


FIG. S3. Method for extracting the field positions of the CF GR is shown for six different densities $n$ indicated in units of $10^{10}$ cm$^{-2}$. First a parabolic background (orange curve) is obtained from fitting the raw data (black traces) to a second-order polynomial. Then that background is subtracted from the data to obtain the purple curves which show the positions of the GRs more clearly. Vertical (dash-dotted) blue, (solid) red, (short-dashed) green, and (long-dashed) brown lines mark the expected positions for the $i = 1$ GR for fully spin-polarized CFs according to the fixed-density model, minority-carrier model, Dirac, and Halperin-Lee-Read theories, respectively. Note that the blue and red lines coincide for $\nu < 1/2$ ($B^* > 0$). The experimental data best match the predictions of the minority-carrier model (red vertical lines). The differences between the observed minima positions and the predictions from the fixed-density model, Dirac, and Halperin-Lee-Read theories are also clearly visible.

(E) When plotted against $a/l_B$, $\nu_{\mathrm{GR}}$ [Fig. S2(c)] and $k_F^*$ [Fig. S2(b)] exhibit mirror symmetry about $\nu = 1/2$. However, $B_{i=1}^*$, even if plotted as a function of $a/l_B$, exhibit asymmetry between the locations of $B^+$ and $B^-$ about $B_{\nu=1/2}$ [Fig. S2(d)] ; this is because $B_{\nu=1/2}$ (also $n$) is different for $B^* > 0$ and $B^* < 0$ when $a/l_B$ is fixed which, according to Eqs. (S10), (S13), and (S16), will cause $|B^{*+}| = |B^+ - B_{\nu=1/2}|$ and $|B^{*-}| = |B^- - B_{\nu=1/2}|$ to be not equal at a fixed $a/l_B$.

(F) There are discontinuities in the $k_F^*$ [Fig. S2(b)] and $B_{i=1}^*$ [Fig. S2(d)] data when plotted against $a/l_B$. The discontinuities stem from the two different superlat-

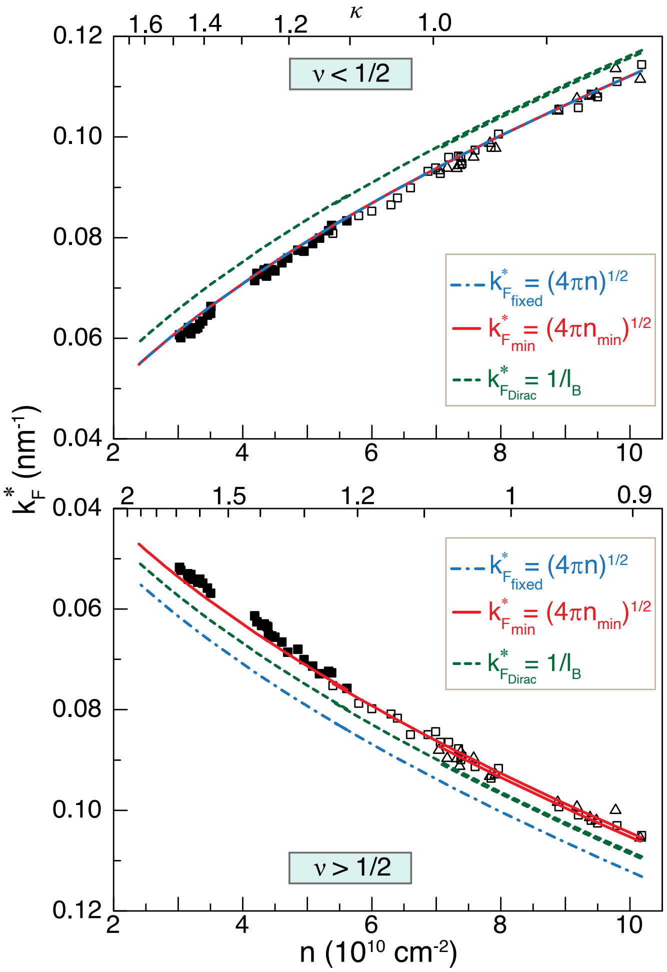


FIG. S4. A plot similar to Fig. 3 of the main text, showing the measured CF Fermi wave vectors from the $i = 1$ GR minimum directly obtained from the raw data without any background subtraction. Blue, red, and green curves represent the calculated $k^*_F$ based on $k^*_F = (4\pi n)^{1/2}$, $k^*_F = (4\pi n_{\rm min})^{1/2}$, and Dirac theory, respectively. The experimental data match best with $k^*_F = (4\pi n_{\rm min})^{1/2}$.

tice periods $a$ that we use in the measurements. In Fig. S2(b), since $k^*_F$ is independent of the superlattice periods $a$, when the data is plotted against $a/l_B$, a discontinuity arises because of the discontinuous $a$ values (190 and 200 nm). As also seen in Eqs. (S1), (S10), (S13), and (S16), $B^*_{i=1}$ and the corresponding $l_B$ depend on $a$ and $B_{\nu=1/2}$ ($n$). Therefore, to obtain $B^*_{i=1}$ at a fixed $a/l_B$, $B_{\nu=1/2}$ needs to be different on the two sides of $B^* = 0$; this difference is dependent on $a$. Thus a sudden change in $a$ (190 to 200 nm) creates a discontinuity in the $B^*_{i=1}$ plots in Fig. S2(d). This is not the case in $\nu_{\rm GR}$ plots [see Figs. 4 and S2(c)] because, unlike $B_{\nu=1/2}$, $\nu_{\nu=1/2}$ is a constant and always equal to 1/2.

## V. DATA ANALYSIS

At very low electron densities, the GR resistance minima on the flanks of $\nu = 1/2$ are sometimes masked by the rapidly changing background resistance (see the black traces in Fig. S3), expected from a weak one-dimensional modulation near $\nu = 1/2$ [17]. We note that a quadratic background near $\nu = 1/2$, i.e. the positive magneto-resistance at small $|B^*|$, is attributed to open orbits of CFs, analogous to the open orbits of carriers of the classical magnetic breakdown mechanism; see Refs. [1, 13]. This rising background continues even at $|B^*|$ values beyond the locations of the $i = 1$ CF GR features. Therefore, to accurately extract the positions of the GR features, we perform a background subtraction process. First, we fit the data to a second-order polynomial to obtain a smooth parabolic background (orange curves in Fig. S3). Then we subtract that background from the data to obtain more pronounced GR minima (purple traces in Fig. S3), and extract their magnetic field positions with greater accuracy. Inevitably, there is noise present in the data. Therefore, the minima positions are extracted after smoothing the data near the minima.

To cross-check with the raw data and further appreciate the accuracy of our GR data in distinguishing between the predictions of the different theoretical models, in Fig. S3 we mark the locations of the $i = 1$ CF GR minima expected from different theoretical models with color-coded vertical lines. Blue, red, green and brown vertical lines denote the locations of the $i = 1$ CF GR minima predicted by the fixed-density model, minority-carrier model, Dirac, and Halperin-Lee-Read theories, respectively.

It is clear in the Fig. S3 traces that the observed GR resistance minima match the red vertical lines (minority-carrier model) best, and that the other models show obvious deviations from the experimental data. The agreement of the markings with both the unprocessed ("raw") data and the background-subtracted data is also very reasonable. We note that for the high-density traces, e.g. $n = 10.16$ and 7.94 traces in Figs. 2(c, d) of the main text, no background subtraction is needed because the CF GR resistance minima are well pronounced at high densities.

We also show a summary of $k^*_F$ obtained from the unprocessed data plotted against density in Fig. S4. Figure S4 is similar to Fig. 3 of the main text except that here the $k^*_F$ values are obtained directly from the unprocessed data. Despite a slightly more pronounced scatter among the data points, they still match more closely the $k^*_F = (4\pi n_{\rm min})^{1/2}$ curves rather than $k^*_F = (4\pi n)^{1/2}$ or the $k^*_F = 1/l_B$ curves.

[1] D. Kamburov, Y. Liu, M. A. Mueed, M. Shayegan, L. N. Pfeiffer, K. W. West, and K. W. Baldwin, What Determines the Fermi Wave Vector of Composite Fermions? Phys. Rev. Lett. **113**, 196801 (2014).

[2] M. A. Mueed, Md. S. Hossain, L. N. Pfeiffer, K. W. West, K. W. Baldwin, and M. Shayegan, Reorientation of the Stripe Phase of 2D Electrons by a Minute Density Modulation, Phys. Rev. Lett. **117**, 076803 (2016).

[3] Md. S. Hossain, M. K. Ma, M. A. Mueed, L. N. Pfeiffer, K. W. West, K. W. Baldwin, and M. Shayegan, Direct Observation of Composite Fermions and Their Fully-Spin-Polarized Fermi Sea Near $\nu = 5/2$, Phys. Rev. Lett. **120**, 256601 (2018).

[4] N. E. Hussey, M. Abdel-Jawad, A. Carrington, A. P. Mackenzie, and L. Balicas, A coherent three-dimensional Fermi surface in a high-transition-temperature superconductor, Nature (London) **425**, 814 (2003).

[5] M. Platé, J. D. F. Mottershead, I. S. Elfimov, D. C. Peets, R. Liang, D. A. Bonn, W. N. Hardy, S. Chiuzbaian, M. Falub, M. Shi, L. Patthey, and A. Damascelli, Fermi Surface and Quasiparticle Excitations of Overdoped $Tl_2Ba_2CuO_{6+\delta}$, Phys. Rev. Lett. **95**, 077001 (2005).

[6] N. Doiron-Leyraud, C. Proust, D. LeBoeuf, J. Levallois, J. -B. Bonnemaison, R. Liang, D. A. Bonn, W. N. Hardy, and L. Taillefer, Quantum oscillations and the Fermi surface in an underdoped high-$T_c$ superconductor, Nature (London) **447**, 565 (2007).

[7] J. K. Jain, *Composite fermions* (Cambridge University Press, New York, 2007).

[8] J. Zhao, Y. Zhang, and J. K. Jain, Crystallization in the Fractional Quantum Hall Regime Induced by Landau-Level Mixing, Phys. Rev. Lett. **121**, 116802 (2018).

[9] J. K. Jain, Composite-Fermion Approach for the Fractional Quantum Hall Effect, Phys. Rev. Lett. **63**, 199 (1989).

[10] B. I. Halperin, P. A. Lee, and N. Read, Theory of the half-filled Landau level, Phys. Rev. B **47**, 7312 (1993).

[11] R. L. Willett, R. R. Ruel, K. W. West, and L. N. Pfeiffer, Experimental Demonstration of a Fermi Surface at One-Half Filling of the Lowest Landau Level, Phys. Rev. Lett. **71**, 3846 (1993).

[12] W. Kang, H. L. Stormer, L. N. Pfeiffer, K. W. Baldwin, and K. W. West, How Real are Composite Fermions? Phys. Rev. Lett. **71**, 3850 (1993).

[13] J. H. Smet, S. Jobst, K. von Klitzing, D. Weiss, W. Wegscheider, and V. Umansky, Commensurate Composite Fermions in Weak Periodic Electrostatic Potentials: Direct Evidence of a Periodic Effective Magnetic Field, Phys. Rev. Lett. **83**, 2620 (1999).

[14] R. L. Willett, K. W. West, and L. N. Pfeiffer, Geometric Resonance of Composite Fermion Cyclotron Orbits with a Fictitious Magnetic Field Modulation, Phys. Rev. Lett. **83**, 2624 (1999).

[15] A. K. C. Cheung, S. Raghu, and M. Mulligan, Weiss oscillations and particle-hole symmetry at the half-filled Landau level, Phys. Rev. B **95**, 235424 (2017).

[16] A. Mitra and M. Mulligan, Fluctuations and magnetoresistance oscillations near the half-filled Landau level, Phys. Rev. B **100**, 165122 (2019).

[17] S. D. M. Zwerschke and R. R. Gerhardts, Positive Magnetoresistance of Composite Fermion Systems with a Weak One-Dimensional Density Modulation, Phys. Rev. Lett. **83**, 2616 (1999).
